# Supplementary material for: Bilateral Self-unbiased Learning from Biased Implicit Feedback
Source: arXiv:2207.12660 source file (2022-07-26)
Supplement: Supplementary file 1 [file sec-appendix.tex]

\newpage
\appendix

\begin{figure}[t!]
\centering
\begin{tabular}{cc}
\includegraphics[width=0.21\textwidth]{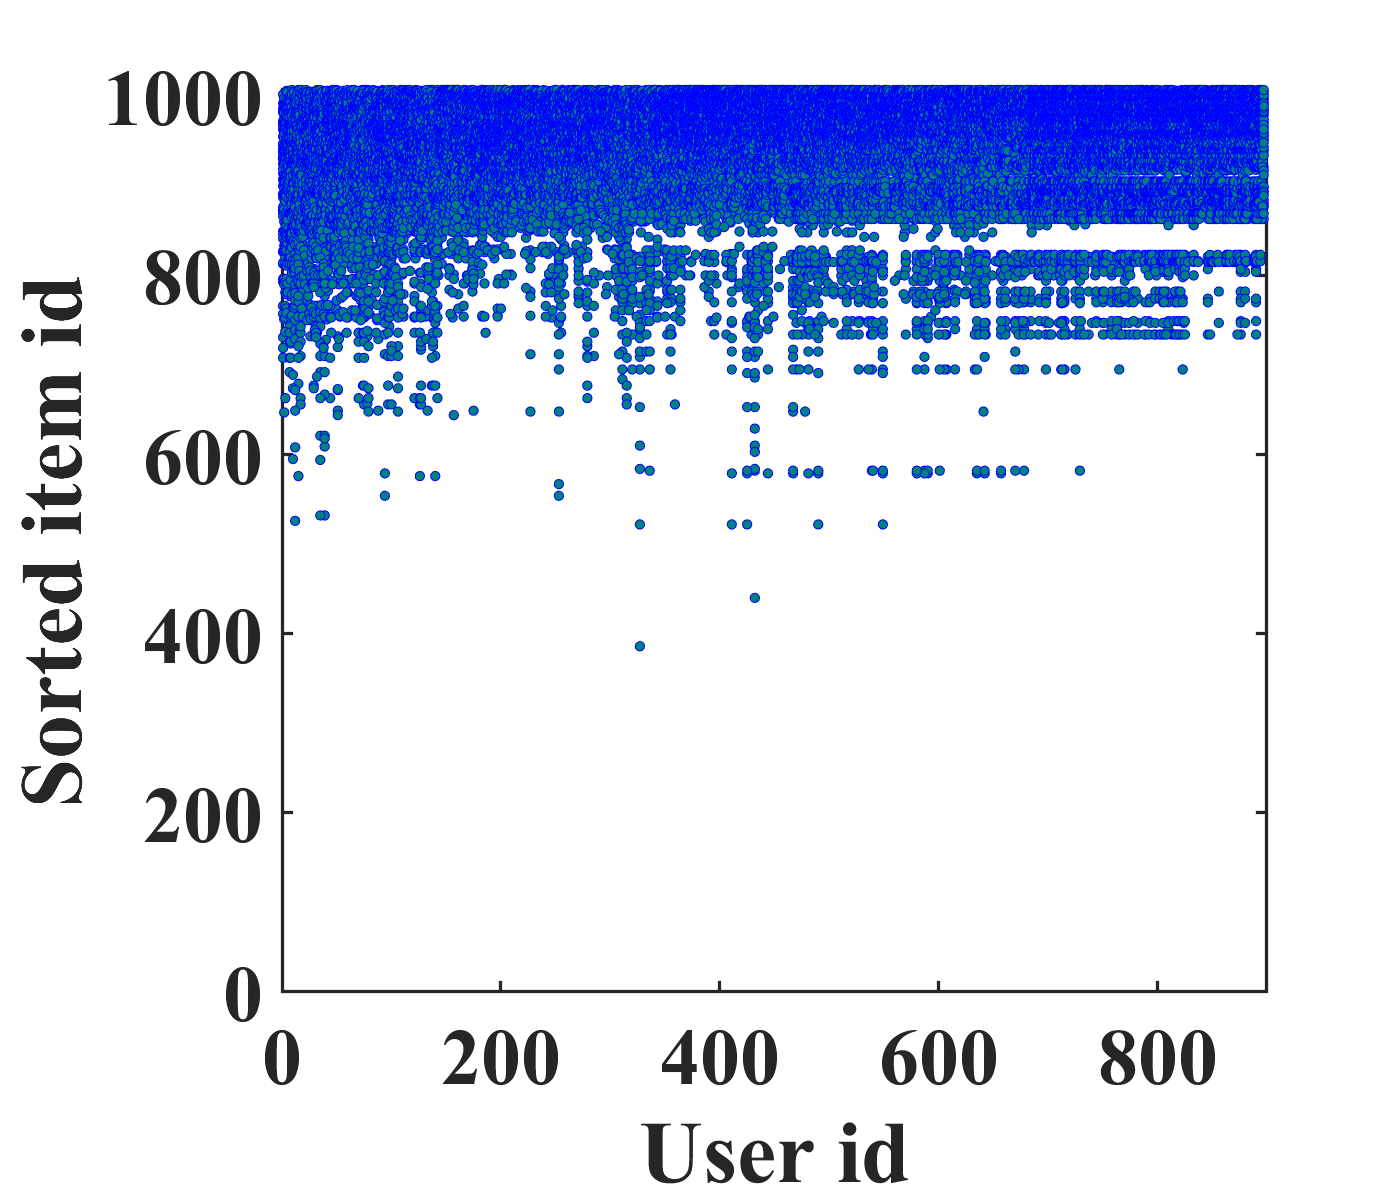} &
\includegraphics[width=0.21\textwidth]{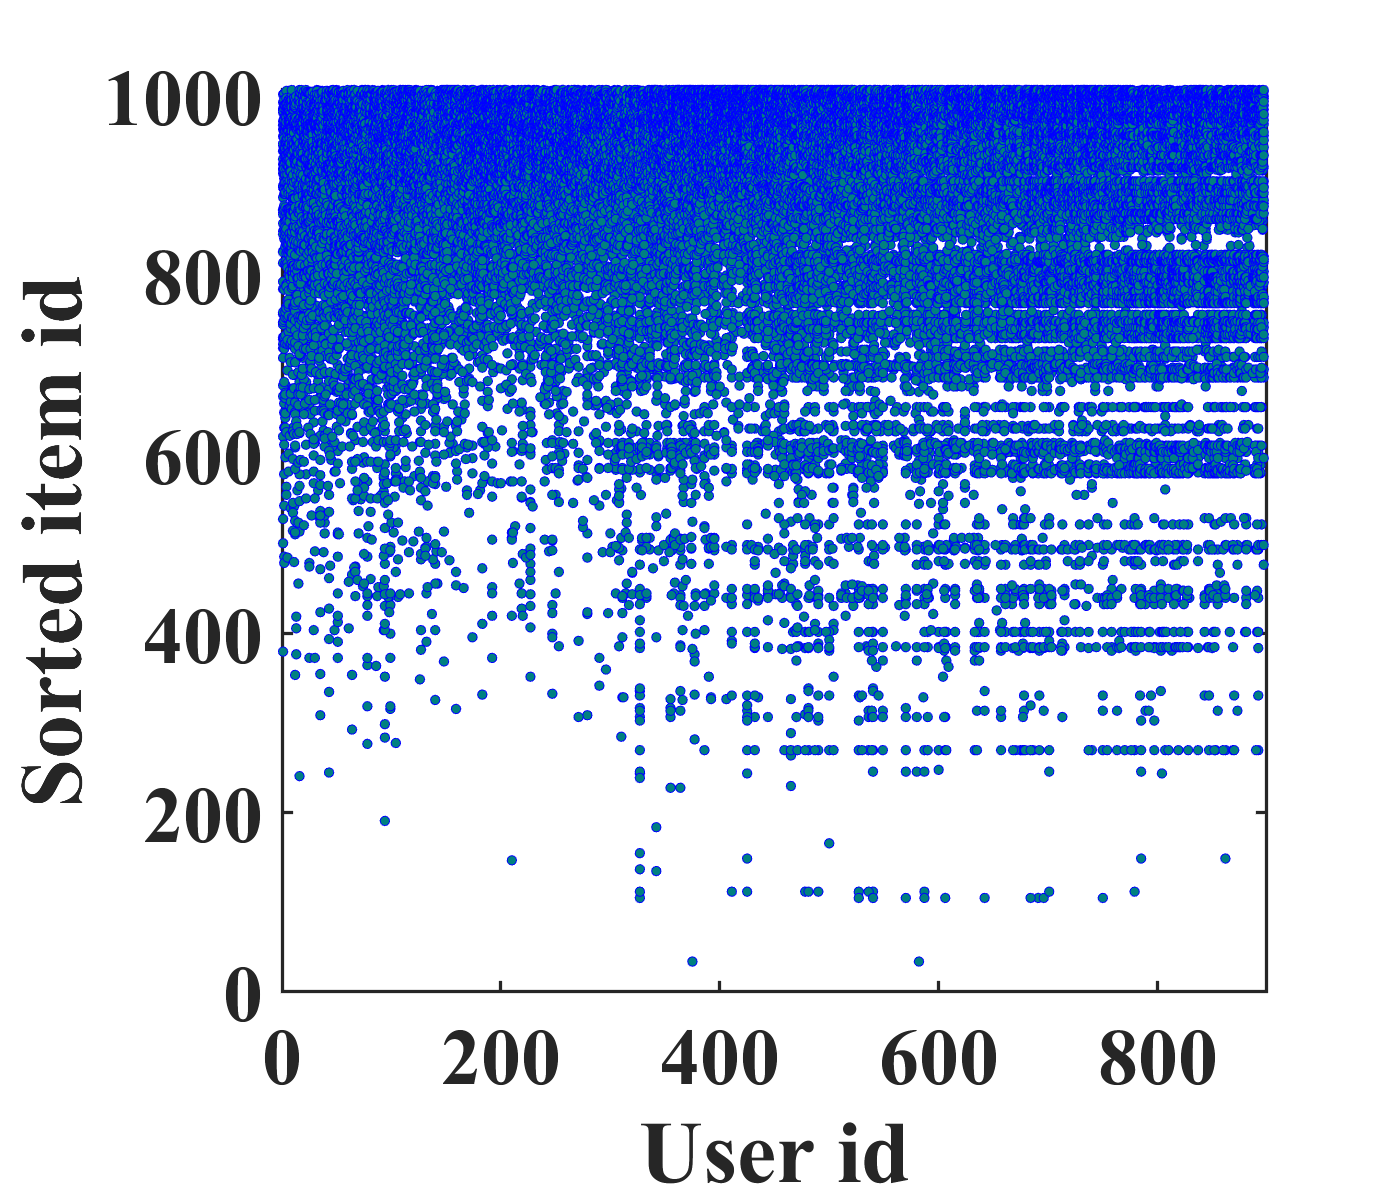} \\
\multicolumn{1}{c}{(a) MF} &\multicolumn{1}{c}{(b) Unbiased MF (ours)}
% \vspace{4mm}
\end{tabular}
\caption{Item distributions for MF and our Unbiased MF on ML-100K. All items are top-50 recommended items for each user. The y-axis means that the sorted item id by item popularity. That is, the larger the item id, the more popular it is. While MF mainly recommends popular items, the unbiased MF recommends more diverse items.}\label{fig:mf_self}
%\vskip -1.5
\end{figure}
